# Supplementary material for: UniSRM: A Unified Speech Reward Model for Reasoning-Based Fine-grained Assessment
Source: arXiv:2605.23261 source file (2026-05-22)
Supplement: Supplementary file 1 [file related_works.tex]

\section{Related Works}
\subsection{Multimodal Reward Models}

Reinforcement learning from human feedback (RLHF) and its variants have become an effective paradigm for aligning large language models (LLMs) with human preferences~\citep{ziegler2019fine,ouyang2022training,rafailov2023direct}. Recent works extend this paradigm to multimodal settings, where reward models provide supervisory signals for both understanding and generation tasks over image, video, and audio~\citep{team2023gemini,lee2023aligning, wang2024lift,liu2025improving,zhao2025omnialign, wang2025unified}.
Early reward models, while effective to some extent, are mostly trained as scalar regressors on preference supervision. Such models typically produce shallow or implicit reasoning without explicit reasoning traces, which often leads to unreliable or unstable reward signals in complex scenarios and can yield incorrect conclusions due to flawed reasoning processes.
Recent work has begun addressing these limitations by incorporating explicit reasoning. HumanOmniV2~\citep{yang2025humanomniv2} advances omni-modal LLMs by multi-step reasoning across modalities, showing that stronger understanding naturally supports complex human intentions and emotions. UnifiedReward-Think~\citep{wang2025unified} leverages reinforcement learning to activate and
enhance Visual-Language Models (VLMs)' latent reasoning capabilities demonstrates that explicit long CoT significantly can strengthen reasoning quality and accuracy.
However, despite this progress in multimodal settings, reward modeling for speech still has meaningful room for further improvement.
% Existing speech reward models still rely heavily on single-dimensional signal-based metrics or lack transparent, structured reasoning, making it difficult to capture the inherently multi-faceted nature of human speech perception. This gap highlights the need for a dedicated, interpretable, and multi-dimensional reward framework tailored specifically to speech generation.

\subsection{Speech Reward Models}
\subsubsection{Classical Speech Reward Signals}
Traditional speech generation systems are primarily evaluated with subjective Mean Opinion Score (MOS) tests \cite{ITU-T_P800_1996}, where human raters assign scalar scores to perceived quality or naturalness. While MOS remains the gold standard, it is expensive, slow, and difficult to standardize across datasets and labs, resulting in noisy optimization targets. To alleviate these issues, many works adopt automatic, signal-based metrics such as word error rate (WER), speaker similarity (SIM), PESQ, DNSMOS, and UTMOS~\citep{saeki2022utmos}. These metrics capture specific aspects of quality (e.g., transcription accuracy, speaker timbre, or naturalness) and have been used as reward signals in RL-based text-to-speech optimization~\cite{zhang2024speechalign, fu2024asrrl, hu2024robust, sun2025f5r, chen2025fine}.

However, all these indicators are inherently single-dimensional. For instance, WER focuses on semantic correctness, SIM measures timbre similarity, and UTMOS approximates overall naturalness. 
When used as scalar rewards, they fail to provide holistic, human-like judgments and offer no explicit explanation of \emph{why} a sample is preferred. Moreover, combining multiple scalar metrics often requires hand-crafted weighting and still yields opaque reward signals. 

\subsubsection{AudioLLMs as Judges} 
% ATT~\cite{wang2025audio} proposes human-likeness and a multi-dimensional Chinese corpus.
% ALLD~\cite{chen2025audio} first natural-language-based speech evaluation corpus and teaches audio LLMs to describe and score speech quality in a human-like way.
% QualiSpeech~\cite{wang2025qualispeech} also constructs a speech dataset with detailed natural-language reasoning for the low-level quality assessment.
% Meanwhile, SageLM~\cite{ge2025sagelm} and WavReward~\cite{ji2025wavreward} extend LAMs-based evaluators toward speech dialogue interaction
% % 目标是提升对instruction-following能力和对话理解能力的评估

% AudioJudge~\cite{manakul2025audiojudge} investigates prompting strategies to obtain multi-aspect evaluations of lexical content, speech quality, and paralinguistic attributes.

% SpeechLLM-as-Judges~\citep{wang2025speechllm} goes a step further by fine-tuning a speech quality LLM (SQ-LLM) on a large-scale SpeechEval dataset with four tasks.

% SpeechJudge~\citep{zhang2025speechjudge} constructs a large-scale pairwise preference corpus for naturalness and trains a generative reward model with chain-of-thought supervision. While effective for naturalness ranking, SpeechJudge primarily focuses on pairwise comparison and targets TTS generation, lacking support for dialogue-aware contextual evaluation. 

Using audio large language models (audioLLMs) as automated speech judges has recently received growing attention.
ATT~\cite{wang2025audio} and ALLD~\cite{chen2025audio} both introduce a human-likeness speech evaluation corpus and train AudioLLMs to describe and score speech quality in a human-aligned manner. 
QualiSpeech~\cite{wang2025qualispeech} develops a detailed dataset for low-level speech quality assessment. 
AudioJudge~\cite{manakul2025audiojudge} explores prompting strategies to elicit multi-aspect judgments.
WavReward~\cite{ji2025wavreward} extends AudioLLMs to evaluate both IQ and EQ for spoken dialogue systems, but is restricted to single-turn dialogue. SageLM~\cite{ge2025sagelm} also trains an end-to-end spoken dialogue evaluator via SFT for single-turn conversational quality. 
SpeechLLM-as-Judges~\cite{wang2025speechllm} fine-tunes a speech quality LLM on a large-scale SpeechEval dataset to perform assessment, comparison, improvement suggestion, and deepfake detection. 
SpeechJudge~\cite{zhang2025speechjudge} trains a generative reward model primarily centered on naturalness, aiming at utterance-level preference evaluation over paired speech samples.

Some of these above approaches offer evaluation dimensions that are not sufficiently fine-grained and comprehensive~\cite{wang2025audio,chen2025audio,wang2025qualispeech}, while others inherently inherit the limited understanding capacity of the underlying LAMs and may therefore produce shallow judgments~\cite{manakul2025audiojudge}, and some are restricted by insufficient coverage of task scenarios~\cite{wang2025speechllm,zhang2025speechjudge,ge2025sagelm,ji2025wavreward}. 
Moreover, rule-based reinforcement learning lacks supervision over the reasoning process, which can lead to inconsistency between the rationale and final result~\cite{ge2025sagelm, zhang2025speechjudge}. 

Overall, existing audioLLM-based judges still have substantial room for improvement.
In this paper, we propose an end-to-end speech reward model, UniSRM, that decomposes speech quality into multiple complementary dimensions and generates explicit reasoning traces before producing an aggregated preference decision, thus offering both a richer supervision signal and improving interpretability.
To improve the robustness and rationality of the reasoning process, we introduce a fine-grained optimization strategy by adding appropriate supervision. 
Furthermore, our UniSRM covers tasks from utterance-level quality to context-level coherency, including utterance-level speech preference judgments and quality assessment, as well as scenario-aware and dialogue-aware contextual preference evaluations.
