# Supplementary material for: UniSRM: A Unified Speech Reward Model for Reasoning-Based Fine-grained Assessment
Source: arXiv:2605.23261 source file (2026-05-22)
Supplement: Supplementary file 2 [file uniSRM_data.tex]

\section{UniSRM-Data}
\label{sec:data}
We construct \textsc{UniSRM-Data}, a unified dataset that covers speech evaluation tasks ranging
\textit{from utterance-level quality to context-level coherency}, including:
(i) utterance-level speech A/B preference judgment,
(ii) fine-grained utterance-level speech quality assessment,
(iii) scenario-aware style consistency evaluation conditioned on textual context, and
(iv) multi-turn dialogue speech evaluation conditioned on dialogue history.
\paragraph{Task 1: Utterance-Level A/B Preference Judgment.}
% Consistency构造数据法: 引用文章《J1: Incentivizing Thinking in LLM-as-a-Judge via Reinforcement Learning》，两两组合的情况下，打分标准要一致，来筛选数据，保持推理一致；同时训练时，顺序完全随机打乱，避免reward model学到不同分布数据的先后位置。
Pairwise preference comparison is often easier and more reliable than absolute scoring for speech quality assessment, as it directly asks which of two speeches of the same target text is better overall, which is comparable.

Given a text prompt $x$, we use multiple open-source TTS models $s$ to synthesize diverse candidate speech signals.
\begin{equation}
\label{eq1}
    \mathcal{S}(x)=\{ s_{1}, s_{2}, \dots, s_{K} \},
\end{equation}
where $K$ is the number of open-source TTS models.
These speech samples, generated from the same textual content by different synthesis models, are paired to form comparison candidates. 
We additionally include the ground-truth recording $S^{\text{GT}}$ as another candidate. We then form unordered comparison pairs:
\begin{equation}
\begin{aligned}
\mathcal{P}(x)
= \Bigl\{ (s_A, s_B) \;\Bigm|\;&
s_A, s_B \in \mathcal{S}(x)\cup\{S^{\text{GT}}\}, \\
& s_A \neq s_B
\Bigr\}.
\end{aligned}
\end{equation}

To obtain preference annotations, we employ Gemini-2.0-Flash to generate
\emph{multi-dimensional scores and explanations} for each candidate in a pair, covering
ext Fidelity \& Intelligibility, Speaker Similarity,
Prosody \& Expressiveness, and Naturalness \& Audio Quality,
followed by a final binary decision indicating which speech is better.
For each speech sample, Gemini assigns a score in $[0,10]$ for each dimension, and the total score is computed by summation.
The final preference label is determined by comparing the total scores:
\begin{equation}
    \ell_{better} =
    \begin{cases}
    speech A, & \text{if } T_A > T_B,\\[2pt]
    speech B, & \text{otherwise}.
    \end{cases}
\end{equation}
This process yields a high-quality dataset of speech preference pairs for speech reward modeling.

To prevent the reward model from memorizing positional cues, we randomly shuffle the order of $(s_A, s_B)$ for every pair,
so that the first and second positions carry no deterministic meaning.
Since automatic judgments may still contain noise, we further remove self-contradictory samples
by filtering cyclic conflicts, e.g., $A>B,\, B>C,\, C>A$ within the same text group.

Finally, we split all annotated pairs into three disjoint subsets for SFT, GRPO, and Test, ensuring no overlap.
To maximize label reliability for optimization and evaluation, we additionally conduct human verification on the GRPO and Test subsets, retaining only samples aligned with human preference.
The detailed human verification criteria are provided in Appendix~\ref{app:human_verification}.

\paragraph{Task 2: Fine-Grained Utterance-Level Speech Quality Assessment.}
For single-sample speech quality assessment, we directly leverage the public QualiSpeech~\cite{wang2025qualispeech} dataset,
which provides MOS-like annotations across seven perceptual aspects: Noise, Distortion, Speed, Continuity, Naturalness, Listening effort, and Overall quality (each in $[1,5]$).

To align with our reasoning-based training format, we treat QualiSpeech's textual rationales as the model's intermediate reasoning.
Specifically, the aspect descriptions, 
Noise description, Distortion description, Unnatural pause, Feeling of voice, together with a
Natural language description are used as the reasoning trace,
while the seven aspect scores are used as the final structured answer.
This design enables UniSRM to learn fine-grained, interpretable quality assessment rather than a black-box scalar prediction.

\paragraph{Task 3: Scenario-Aware Style Consistency under Textual Context.}
Speech quality cannot always be judged from an isolated utterance: in expressive narration or voice acting, the speech must match the scene context and target emotion.
To this end, we define a new task, scenario-aware style consistency evaluation conditioned on textual context,
and construct bilingual data using the Emotional Speech Dataset (ESD)\citep{zhou2022esd}.

For each ESD utterance, we treat the original recording as a positive sample.
We then call GPT-4.1~\citep{openai2024gpt4technicalreport} to generate a coherent scenario description and paragraph context
conditioned on the utterance text and emotion label, ensuring that the context naturally leads to the target sentence
and makes the emotion plausible. These two fields serve as the textual context to be conditioned on during evaluation.

To construct hard negatives, we sample one negative type per instance with predefined probabilities.
Negatives are created either by selecting real ESD recordings or by synthesizing speech using open-source TTS systems, e.g., CosyVoice2, F5-TTS, ChatTTS, XTTS. The negative construction includes:
\begin{itemize}[leftmargin=1.5em, nosep]
    \item Real-speech negatives from ESD with the same text but different emotion, different text and different emotion, or different text but same emotion;
    \item Synthesized negatives using open-source TTS models, where we optionally generate a mismatching negative text via GPT-4.1 conditioned on the same scenario context, and TTS models synthesize speech accordingly.
\end{itemize}

For TTS-based negatives, we assign prompt speech from ESD and LibriTTS-R.
When the prompt is drawn from ESD, we enforce different emotion from the positive to strengthen the negative signal.
We also randomize controllable attributes supported by each TTS system, e.g., role, speaking rate, and emotion style,
to increase diversity, while explicitly filtering to avoid accidentally matching the positive emotion.

Our constructed pairs explicitly encode which sample is intended to be context-consistent.
Based on prior knowledge of which speech is better, we use Gemini-2.5-Pro to produce multi-dimensional scores and explanations under the given scenario context,
including Text Fidelity, Scenario Style Match, Naturalness \& Audio Quality, together with a final A/B decision.
We build both English and Chinese variants by generating bilingual contexts and prompts,
resulting in a bilingual scenario-aware evaluation set.

\paragraph{Task 4: Multi-Turn Dialogue Speech Evaluation under Dialogue History.}
Existing speech reward modeling for dialogue is often limited to single-turn settings.
We first construct a multi-turn dialogue speech evaluation task conditioned on the dialogue history audio,
enabling reward modeling of dialogue-level consistency.

We choose the DailyTalk \citep {lee2022dailytalk} as basic dialogue dataset.
For each dialogue, we randomly select a target turn $T$ as the current response and use the concatenation of all previous turns
$\{1,\dots,t-1\}$ as the spoken dialogue history.
The original turn $T$ speech is treated as a positive candidate; additionally, we synthesize a portion of positives
using the same TTS engines as negatives to reduce shortcut learning from recording conditions, e.g., \textit{``real vs.\ synthesized''}.

We construct negatives along two complementary axes: text errors and audio errors, and sample from three categories:
\begin{itemize}[leftmargin=1.5em, nosep]
    \item Text-only negatives: 
    keep speaker style as consistent as possible, but generate an inappropriate response text for turn $t$
    using GPT-4.1 conditioned on the multi-turn history, with controlled error types such as
    \emph{in-context but wrong intent}, \emph{context contradiction}, \emph{role confusion}, or \emph{over/under-informativeness}.
    These negatives encourage modeling dialogue act and contextual consistency beyond superficial topical mismatch.
    \item Audio-only negatives:
    keep the response text fixed but alter audio factors, e.g., using an incorrect prompt speaker
    (speaker swap within the dialogue or sampling an unseen speaker from LibriTTS-R),
    or manipulating prosody/emotion to violate the dialogue context.
    These negatives emphasize speaker consistency and prosody/emotion match.
    \item Mixed negatives:
    Both text and audio are mismatched to encourage holistic robustness.
\end{itemize}

All positive and negative responses are synthesized with multiple open-source TTS models
(CosyVoice2, F5-TTS, ChatTTS, XTTS) for diversity.
Finally, given the dialogue history audio and the two candidate responses,
we use Gemini-2.5-Pro to produce multi-dimensional scores and reasoning across Intent Matching, Speaker Consistency, Contextual Consistency, Emotion, and Overall Naturalness,
followed by an overall A/B decision.

Finally, we split the \textsc{UniSRM-Data} into supervised training, RL training, and test sets, denoted as $\mathcal{D}_{\text{SFT}}$ and $\mathcal{D}_{\text{GRPO}}$, respectively, with the test set referred to as \textsc{UniSRM-Bench}.
